# Supplementary material for: Identifying the Source of Vulnerability in Explanation Discrepancy: A Case Study in Neural Text Classification
Source: arXiv:2212.05327 source file (2022-12-10)
Supplement: Supplementary file 2 [file tables.tex]

% SST2
\begin{table}[htbp]
\centering
\begin{tabular}{llll}
\hline
\textbf{Dataset} & \textbf{Perturbation} & \textbf{Level}& \textbf{$\sigma^{2}$} \\
% \hline
    %   & & & CNN & LSTM & BERT \\
\hline
SST-2  & Input ($\sigma^{2}_{input}$)& 0 & 0 \\
      & & 1 & 0.05 \\
      & & 2 & 0.1 \\
      & & 3 & 0.15 \\
      & & 4 & 0.2 \\
\hline
      & Output ($\sigma^{2}_{output}$)& 0 & 0  \\
      & & 1 & 0.25 \\
      & & 2 & 0.5 \\
      & & 3 & 0.75 \\
      & & 4 & 1 \\
\hline
\end{tabular}
\caption{Perturbation levels applied on the SST-2 dataset}
\label{tab:4}
\end{table}

% AG
\begin{table}[htbp]
\centering
\begin{tabular}{llll}
\hline
\textbf{Dataset} & \textbf{Perturbation} & \textbf{Level}& \textbf{$\sigma^{2}$} \\
% \hline
    %   & & & CNN & LSTM & BERT \\
\hline
AG's News  & Input ($\sigma^{2}_{input}$)& 0 & 0 \\
      & & 1 & 0.05 \\
      & & 2 & 0.1 \\
      & & 3 & 0.15 \\
      & & 4 & 0.2 \\
\hline
      & Output ($\sigma^{2}_{output}$)& 0 & 0  \\
      & & 1 & 0.25 \\
      & & 2 & 0.5 \\
      & & 3 & 0.75 \\
      & & 4 & 1 \\
\hline
\end{tabular}
\caption{Perturbation levels applied on the AG's News dataset}
\label{tab:5}
\end{table}

% TREC
\begin{table}[htbp]
\centering
\begin{tabular}{llll}
\hline
\textbf{Dataset} & \textbf{Perturbation} & \textbf{Level}& \textbf{$\sigma^{2}$} \\
% \hline
    %   & & & CNN & LSTM & BERT \\
\hline
TREC  & Input ($\sigma^{2}_{input}$)& 0 & 0 \\
      & & 1 & 0.05 \\
      & & 2 & 0.1 \\
      & & 3 & 0.15 \\
      & & 4 & 0.2 \\
\hline
      & Output ($\sigma^{2}_{output}$)& 0 & 0  \\
      & & 1 & 0.25 \\
      & & 2 & 0.5 \\
      & & 3 & 0.75 \\
      & & 4 & 1 \\
\hline
\end{tabular}
\caption{Perturbation levels applied on the TREC dataset}
\label{tab:6}
\end{table}
